# Supplementary material for: Off the Driven Path: Transferable Road Understanding in Driving VLAs
Source: arXiv:2611.33878 source file (2026-11-25)
Supplement: Supplementary file 1 [file geo_balanced.tex]

\qsseg{0}{0.000}{48.757}{0.64}{1.36}%
\qsseg{1}{49.107}{96.079}{0.64}{1.36}%
\qsseg{2}{96.429}{100.000}{0.64}{1.36}%
\qsseg{0}{0.000}{54.367}{1.64}{2.36}%
\qsseg{1}{54.717}{100.000}{1.64}{2.36}%
\qsseg{0}{0.000}{34.785}{2.64}{3.36}%
\qsseg{1}{35.135}{69.920}{2.64}{3.36}%
\qsseg{2}{70.270}{92.443}{2.64}{3.36}%
\qsseg{1}{92.793}{100.000}{2.64}{3.36}%
\qsseg{0}{0.000}{42.919}{3.64}{4.36}%
\qsseg{1}{43.269}{82.342}{3.64}{4.36}%
\qsseg{2}{82.692}{100.000}{3.64}{4.36}%
\qsseg{0}{0.000}{51.436}{4.64}{5.36}%
\qsseg{1}{51.786}{100.000}{4.64}{5.36}%
\qsseg{0}{0.000}{3.496}{5.64}{6.36}%
\qsseg{1}{3.846}{7.342}{5.64}{6.36}%
\qsseg{2}{7.692}{11.188}{5.64}{6.36}%
\qsseg{1}{11.538}{15.035}{5.64}{6.36}%
\qsseg{2}{15.385}{18.881}{5.64}{6.36}%
\qsseg{1}{19.231}{22.727}{5.64}{6.36}%
\qsseg{2}{23.077}{26.573}{5.64}{6.36}%
\qsseg{1}{26.923}{30.419}{5.64}{6.36}%
\qsseg{2}{30.769}{34.265}{5.64}{6.36}%
\qsseg{1}{34.615}{38.112}{5.64}{6.36}%
\qsseg{2}{38.462}{41.958}{5.64}{6.36}%
\qsseg{1}{42.308}{45.804}{5.64}{6.36}%
\qsseg{2}{46.154}{49.650}{5.64}{6.36}%
\qsseg{1}{50.000}{52.535}{5.64}{6.36}%
\qsseg{2}{52.885}{55.419}{5.64}{6.36}%
\qsseg{1}{55.769}{58.304}{5.64}{6.36}%
\qsseg{2}{58.654}{61.188}{5.64}{6.36}%
\qsseg{1}{61.538}{64.073}{5.64}{6.36}%
\qsseg{2}{64.423}{66.958}{5.64}{6.36}%
\qsseg{1}{67.308}{69.842}{5.64}{6.36}%
\qsseg{2}{70.192}{72.727}{5.64}{6.36}%
\qsseg{1}{73.077}{75.612}{5.64}{6.36}%
\qsseg{2}{75.962}{78.496}{5.64}{6.36}%
\qsseg{1}{78.846}{80.419}{5.64}{6.36}%
\qsseg{2}{80.769}{82.342}{5.64}{6.36}%
\qsseg{1}{82.692}{84.265}{5.64}{6.36}%
\qsseg{2}{84.615}{86.188}{5.64}{6.36}%
\qsseg{1}{86.538}{88.112}{5.64}{6.36}%
\qsseg{2}{88.462}{90.035}{5.64}{6.36}%
\qsseg{1}{90.385}{91.958}{5.64}{6.36}%
\qsseg{2}{92.308}{93.881}{5.64}{6.36}%
\qsseg{1}{94.231}{95.804}{5.64}{6.36}%
\qsseg{2}{96.154}{96.765}{5.64}{6.36}%
\qsseg{1}{97.115}{97.727}{5.64}{6.36}%
\qsseg{2}{98.077}{98.688}{5.64}{6.36}%
\qsseg{1}{99.038}{100.000}{5.64}{6.36}%
\qsseg{0}{0.000}{50.559}{6.64}{7.36}%
\qsseg{1}{50.909}{100.000}{6.64}{7.36}%
\qsseg{0}{0.000}{34.265}{7.64}{8.36}%
\qsseg{1}{34.615}{66.958}{7.64}{8.36}%
\qsseg{2}{67.308}{90.035}{7.64}{8.36}%
\qsseg{1}{90.385}{95.804}{7.64}{8.36}%
\qsseg{2}{96.154}{97.727}{7.64}{8.36}%
\qsseg{1}{98.077}{100.000}{7.64}{8.36}%
\qsseg{0}{0.000}{49.650}{8.64}{9.36}%
\qsseg{1}{50.000}{100.000}{8.64}{9.36}%
\qsseg{0}{0.000}{34.693}{9.64}{10.36}%
\qsseg{1}{35.043}{68.881}{9.64}{10.36}%
\qsseg{2}{69.231}{100.000}{9.64}{10.36}%
\qsseg{0}{0.000}{27.607}{10.64}{11.36}%
\qsseg{1}{27.957}{54.489}{10.64}{11.36}%
\qsseg{2}{54.839}{80.295}{10.64}{11.36}%
\qsseg{1}{80.645}{89.973}{10.64}{11.36}%
\qsseg{2}{90.323}{97.499}{10.64}{11.36}%
\qsseg{1}{97.849}{100.000}{10.64}{11.36}%
\qsseg{0}{0.000}{26.065}{11.64}{12.36}%
\qsseg{1}{26.415}{52.480}{11.64}{12.36}%
\qsseg{2}{52.830}{78.895}{11.64}{12.36}%
\qsseg{1}{79.245}{95.876}{11.64}{12.36}%
\qsseg{2}{96.226}{97.763}{11.64}{12.36}%
\qsseg{1}{98.113}{100.000}{11.64}{12.36}%
\qsseg{0}{0.000}{50.077}{12.64}{13.36}%
\qsseg{1}{50.427}{100.000}{12.64}{13.36}%
\qsseg{0}{0.000}{25.291}{13.64}{14.36}%
\qsseg{1}{25.641}{50.932}{13.64}{14.36}%
\qsseg{2}{51.282}{75.718}{13.64}{14.36}%
\qsseg{1}{76.068}{100.000}{13.64}{14.36}%
\qsseg{0}{0.000}{30.126}{14.64}{15.36}%
\qsseg{1}{30.476}{60.602}{14.64}{15.36}%
\qsseg{2}{60.952}{80.602}{14.64}{15.36}%
\qsseg{1}{80.952}{100.000}{14.64}{15.36}%
\qsseg{0}{0.000}{16.457}{15.64}{16.36}%
\qsseg{1}{16.807}{33.263}{15.64}{16.36}%
\qsseg{2}{33.613}{50.070}{15.64}{16.36}%
\qsseg{1}{50.420}{66.877}{15.64}{16.36}%
\qsseg{2}{67.227}{83.684}{15.64}{16.36}%
\qsseg{1}{84.034}{100.000}{15.64}{16.36}%
\qsseg{0}{0.000}{17.722}{16.64}{17.36}%
\qsseg{1}{18.072}{35.795}{16.64}{17.36}%
\qsseg{2}{36.145}{49.048}{16.64}{17.36}%
\qsseg{1}{49.398}{61.096}{16.64}{17.36}%
\qsseg{2}{61.446}{68.325}{16.64}{17.36}%
\qsseg{1}{68.675}{75.554}{16.64}{17.36}%
\qsseg{2}{75.904}{81.578}{16.64}{17.36}%
\qsseg{1}{81.928}{86.397}{16.64}{17.36}%
\qsseg{2}{86.747}{90.011}{16.64}{17.36}%
\qsseg{1}{90.361}{92.421}{16.64}{17.36}%
\qsseg{2}{92.771}{94.831}{16.64}{17.36}%
\qsseg{1}{95.181}{96.036}{16.64}{17.36}%
\qsseg{2}{96.386}{97.240}{16.64}{17.36}%
\qsseg{1}{97.590}{98.445}{16.64}{17.36}%
\qsseg{2}{98.795}{100.000}{16.64}{17.36}%
\qsseg{0}{0.000}{33.263}{17.64}{18.36}%
\qsseg{1}{33.613}{66.877}{17.64}{18.36}%
\qsseg{2}{67.227}{100.000}{17.64}{18.36}%
\qsseg{0}{0.000}{6.989}{18.64}{19.36}%
\qsseg{1}{7.339}{14.329}{18.64}{19.36}%
\qsseg{2}{14.679}{20.751}{18.64}{19.36}%
\qsseg{1}{21.101}{27.173}{18.64}{19.36}%
\qsseg{2}{27.523}{33.595}{18.64}{19.36}%
\qsseg{1}{33.945}{40.017}{18.64}{19.36}%
\qsseg{2}{40.367}{46.439}{18.64}{19.36}%
\qsseg{1}{46.789}{52.861}{18.64}{19.36}%
\qsseg{2}{53.211}{59.283}{18.64}{19.36}%
\qsseg{1}{59.633}{65.705}{18.64}{19.36}%
\qsseg{2}{66.055}{72.127}{18.64}{19.36}%
\qsseg{1}{72.477}{77.632}{18.64}{19.36}%
\qsseg{2}{77.982}{83.136}{18.64}{19.36}%
\qsseg{1}{83.486}{88.641}{18.64}{19.36}%
\qsseg{2}{88.991}{93.228}{18.64}{19.36}%
\qsseg{1}{93.578}{96.898}{18.64}{19.36}%
\qsseg{2}{97.248}{98.733}{18.64}{19.36}%
\qsseg{1}{99.083}{100.000}{18.64}{19.36}%
\qsseg{0}{0.000}{27.952}{19.64}{20.36}%
\qsseg{1}{28.302}{54.367}{19.64}{20.36}%
\qsseg{2}{54.717}{77.952}{19.64}{20.36}%
\qsseg{1}{78.302}{100.000}{19.64}{20.36}%
\qsseg{0}{0.000}{16.317}{20.64}{21.36}%
\qsseg{1}{16.667}{32.057}{20.64}{21.36}%
\qsseg{2}{32.407}{47.798}{20.64}{21.36}%
\qsseg{1}{48.148}{63.539}{20.64}{21.36}%
\qsseg{2}{63.889}{78.354}{20.64}{21.36}%
\qsseg{1}{78.704}{89.465}{20.64}{21.36}%
\qsseg{2}{89.815}{100.000}{20.64}{21.36}%
\qsseg{0}{0.000}{13.628}{21.64}{22.36}%
\qsseg{1}{13.978}{26.532}{21.64}{22.36}%
\qsseg{2}{26.882}{38.360}{21.64}{22.36}%
\qsseg{1}{38.710}{50.188}{21.64}{22.36}%
\qsseg{2}{50.538}{62.016}{21.64}{22.36}%
\qsseg{1}{62.366}{71.693}{21.64}{22.36}%
\qsseg{2}{72.043}{78.145}{21.64}{22.36}%
\qsseg{1}{78.495}{84.596}{21.64}{22.36}%
\qsseg{2}{84.946}{89.973}{21.64}{22.36}%
\qsseg{1}{90.323}{94.274}{21.64}{22.36}%
\qsseg{2}{94.624}{97.499}{21.64}{22.36}%
\qsseg{1}{97.849}{100.000}{21.64}{22.36}%
\qsseg{0}{0.000}{16.997}{22.64}{23.36}%
\qsseg{1}{17.347}{32.303}{22.64}{23.36}%
\qsseg{2}{32.653}{46.589}{22.64}{23.36}%
\qsseg{1}{46.939}{60.874}{22.64}{23.36}%
\qsseg{2}{61.224}{75.160}{22.64}{23.36}%
\qsseg{1}{75.510}{87.405}{22.64}{23.36}%
\qsseg{2}{87.755}{100.000}{22.64}{23.36}%
\qsseg{0}{0.000}{2.012}{23.64}{24.36}%
\qsseg{1}{2.362}{4.374}{23.64}{24.36}%
\qsseg{2}{4.724}{6.737}{23.64}{24.36}%
\qsseg{1}{7.087}{9.099}{23.64}{24.36}%
\qsseg{2}{9.449}{11.461}{23.64}{24.36}%
\qsseg{1}{11.811}{13.823}{23.64}{24.36}%
\qsseg{2}{14.173}{16.185}{23.64}{24.36}%
\qsseg{1}{16.535}{18.548}{23.64}{24.36}%
\qsseg{2}{18.898}{20.910}{23.64}{24.36}%
\qsseg{1}{21.260}{23.272}{23.64}{24.36}%
\qsseg{2}{23.622}{25.634}{23.64}{24.36}%
\qsseg{1}{25.984}{27.996}{23.64}{24.36}%
\qsseg{2}{28.346}{30.359}{23.64}{24.36}%
\qsseg{1}{30.709}{32.721}{23.64}{24.36}%
\qsseg{2}{33.071}{35.083}{23.64}{24.36}%
\qsseg{1}{35.433}{37.445}{23.64}{24.36}%
\qsseg{2}{37.795}{39.807}{23.64}{24.36}%
\qsseg{1}{40.157}{42.170}{23.64}{24.36}%
\qsseg{2}{42.520}{44.532}{23.64}{24.36}%
\qsseg{1}{44.882}{46.894}{23.64}{24.36}%
\qsseg{2}{47.244}{49.256}{23.64}{24.36}%
\qsseg{1}{49.606}{51.619}{23.64}{24.36}%
\qsseg{2}{51.969}{53.981}{23.64}{24.36}%
\qsseg{1}{54.331}{55.556}{23.64}{24.36}%
\qsseg{2}{55.906}{57.130}{23.64}{24.36}%
\qsseg{1}{57.480}{58.705}{23.64}{24.36}%
\qsseg{2}{59.055}{60.280}{23.64}{24.36}%
\qsseg{1}{60.630}{61.855}{23.64}{24.36}%
\qsseg{2}{62.205}{63.430}{23.64}{24.36}%
\qsseg{1}{63.780}{65.004}{23.64}{24.36}%
\qsseg{2}{65.354}{66.579}{23.64}{24.36}%
\qsseg{1}{66.929}{68.154}{23.64}{24.36}%
\qsseg{2}{68.504}{69.729}{23.64}{24.36}%
\qsseg{1}{70.079}{71.304}{23.64}{24.36}%
\qsseg{2}{71.654}{72.878}{23.64}{24.36}%
\qsseg{1}{73.228}{74.453}{23.64}{24.36}%
\qsseg{2}{74.803}{76.028}{23.64}{24.36}%
\qsseg{1}{76.378}{77.603}{23.64}{24.36}%
\qsseg{2}{77.953}{79.178}{23.64}{24.36}%
\qsseg{1}{79.528}{80.752}{23.64}{24.36}%
\qsseg{2}{81.102}{82.327}{23.64}{24.36}%
\qsseg{1}{82.677}{83.902}{23.64}{24.36}%
\qsseg{2}{84.252}{85.477}{23.64}{24.36}%
\qsseg{1}{85.827}{87.052}{23.64}{24.36}%
\qsseg{2}{87.402}{88.626}{23.64}{24.36}%
\qsseg{1}{88.976}{90.201}{23.64}{24.36}%
\qsseg{2}{90.551}{91.776}{23.64}{24.36}%
\qsseg{1}{92.126}{93.351}{23.64}{24.36}%
\qsseg{2}{93.701}{94.926}{23.64}{24.36}%
\qsseg{1}{95.276}{95.713}{23.64}{24.36}%
\qsseg{2}{96.063}{96.500}{23.64}{24.36}%
\qsseg{1}{96.850}{97.288}{23.64}{24.36}%
\qsseg{2}{97.638}{98.075}{23.64}{24.36}%
\qsseg{1}{98.425}{98.863}{23.64}{24.36}%
\qsseg{2}{99.213}{100.000}{23.64}{24.36}%
\qsseg{0}{0.000}{13.112}{24.64}{25.36}%
\qsseg{1}{13.462}{26.573}{24.64}{25.36}%
\qsseg{2}{26.923}{40.035}{24.64}{25.36}%
\qsseg{1}{40.385}{53.496}{24.64}{25.36}%
\qsseg{2}{53.846}{65.035}{24.64}{25.36}%
\qsseg{1}{65.385}{76.573}{24.64}{25.36}%
\qsseg{2}{76.923}{86.188}{24.64}{25.36}%
\qsseg{1}{86.538}{95.804}{24.64}{25.36}%
\qsseg{2}{96.154}{97.727}{24.64}{25.36}%
\qsseg{1}{98.077}{100.000}{24.64}{25.36}%
\qsseg{0}{0.000}{6.793}{25.64}{26.36}%
\qsseg{1}{7.143}{12.915}{25.64}{26.36}%
\qsseg{2}{13.265}{18.017}{25.64}{26.36}%
\qsseg{1}{18.367}{23.119}{25.64}{26.36}%
\qsseg{2}{23.469}{28.221}{25.64}{26.36}%
\qsseg{1}{28.571}{33.323}{25.64}{26.36}%
\qsseg{2}{33.673}{38.426}{25.64}{26.36}%
\qsseg{1}{38.776}{43.528}{25.64}{26.36}%
\qsseg{2}{43.878}{48.630}{25.64}{26.36}%
\qsseg{1}{48.980}{53.732}{25.64}{26.36}%
\qsseg{2}{54.082}{58.834}{25.64}{26.36}%
\qsseg{1}{59.184}{63.936}{25.64}{26.36}%
\qsseg{2}{64.286}{69.038}{25.64}{26.36}%
\qsseg{1}{69.388}{73.119}{25.64}{26.36}%
\qsseg{2}{73.469}{77.201}{25.64}{26.36}%
\qsseg{1}{77.551}{81.283}{25.64}{26.36}%
\qsseg{2}{81.633}{85.364}{25.64}{26.36}%
\qsseg{1}{85.714}{89.446}{25.64}{26.36}%
\qsseg{2}{89.796}{92.507}{25.64}{26.36}%
\qsseg{1}{92.857}{95.568}{25.64}{26.36}%
\qsseg{2}{95.918}{97.609}{25.64}{26.36}%
\qsseg{1}{97.959}{98.630}{25.64}{26.36}%
\qsseg{2}{98.980}{100.000}{25.64}{26.36}%
\qsseg{3}{0.000}{55.506}{28.24}{28.96}%
\qsseg{4}{55.856}{100.000}{28.24}{28.96}%
\qsseg{3}{0.000}{18.234}{29.24}{29.96}%
\qsseg{4}{18.584}{35.933}{29.24}{29.96}%
\qsseg{5}{36.283}{52.747}{29.24}{29.96}%
\qsseg{4}{53.097}{69.562}{29.24}{29.96}%
\qsseg{5}{69.912}{86.376}{29.24}{29.96}%
\qsseg{4}{86.726}{100.000}{29.24}{29.96}%
\qsseg{3}{0.000}{57.594}{30.24}{30.96}%
\qsseg{4}{57.944}{100.000}{30.24}{30.96}%
\qsseg{3}{0.000}{21.555}{31.24}{31.96}%
\qsseg{4}{21.905}{43.460}{31.24}{31.96}%
\qsseg{5}{43.810}{63.460}{31.24}{31.96}%
\qsseg{4}{63.810}{79.650}{31.24}{31.96}%
\qsseg{5}{80.000}{95.840}{31.24}{31.96}%
\qsseg{4}{96.190}{97.745}{31.24}{31.96}%
\qsseg{5}{98.095}{98.698}{31.24}{31.96}%
\qsseg{4}{99.048}{100.000}{31.24}{31.96}%
\qsseg{3}{0.000}{50.070}{32.24}{32.96}%
\qsseg{4}{50.420}{100.000}{32.24}{32.96}%
\qsseg{3}{0.000}{57.448}{33.24}{33.96}%
\qsseg{4}{57.798}{100.000}{33.24}{33.96}%
\qsseg{3}{0.000}{50.085}{34.24}{34.96}%
\qsseg{4}{50.435}{100.000}{34.24}{34.96}%
\qsseg{3}{0.000}{62.150}{35.24}{35.96}%
\qsseg{4}{62.500}{82.983}{35.24}{35.96}%
\qsseg{5}{83.333}{100.000}{35.24}{35.96}%
\qsseg{3}{0.000}{43.881}{36.24}{36.96}%
\qsseg{4}{44.231}{84.265}{36.24}{36.96}%
\qsseg{5}{84.615}{100.000}{36.24}{36.96}%
\qsseg{3}{0.000}{33.563}{37.24}{37.96}%
\qsseg{4}{33.913}{66.607}{37.24}{37.96}%
\qsseg{5}{66.957}{100.000}{37.24}{37.96}%
\qsseg{3}{0.000}{17.297}{38.24}{38.96}%
\qsseg{4}{17.647}{34.944}{38.24}{38.96}%
\qsseg{5}{35.294}{51.751}{38.24}{38.96}%
\qsseg{4}{52.101}{67.717}{38.24}{38.96}%
\qsseg{5}{68.067}{83.684}{38.24}{38.96}%
\qsseg{4}{84.034}{100.000}{38.24}{38.96}%
\qsseg{6}{0.000}{47.522}{40.84}{41.56}%
\qsseg{7}{47.872}{81.565}{40.84}{41.56}%
\qsseg{8}{81.915}{85.820}{40.84}{41.56}%
\qsseg{7}{86.170}{89.012}{40.84}{41.56}%
\qsseg{8}{89.362}{91.139}{40.84}{41.56}%
\qsseg{7}{91.489}{92.203}{40.84}{41.56}%
\qsseg{8}{92.553}{93.267}{40.84}{41.56}%
\qsseg{7}{93.617}{94.331}{40.84}{41.56}%
\qsseg{8}{94.681}{95.395}{40.84}{41.56}%
\qsseg{7}{95.745}{96.459}{40.84}{41.56}%
\qsseg{8}{96.809}{97.522}{40.84}{41.56}%
\qsseg{7}{97.872}{98.586}{40.84}{41.56}%
\qsseg{8}{98.936}{100.000}{40.84}{41.56}%
\qsseg{6}{0.000}{25.206}{41.84}{42.56}%
\qsseg{7}{25.556}{50.761}{41.84}{42.56}%
\qsseg{8}{51.111}{64.094}{41.84}{42.56}%
\qsseg{7}{64.444}{71.872}{41.84}{42.56}%
\qsseg{8}{72.222}{79.650}{41.84}{42.56}%
\qsseg{7}{80.000}{87.428}{41.84}{42.56}%
\qsseg{8}{87.778}{91.872}{41.84}{42.56}%
\qsseg{7}{92.222}{94.094}{41.84}{42.56}%
\qsseg{8}{94.444}{96.317}{41.84}{42.56}%
\qsseg{7}{96.667}{97.428}{41.84}{42.56}%
\qsseg{8}{97.778}{98.539}{41.84}{42.56}%
\qsseg{7}{98.889}{100.000}{41.84}{42.56}%
