# Supplementary material for: Off the Driven Path: Transferable Road Understanding in Driving VLAs
Source: arXiv:2611.33878 source file (2026-11-25)
Supplement: Supplementary file 2 [file geo_natural.tex]

\qsseg{0}{0.000}{91.958}{0.64}{1.36}%
\qsseg{1}{92.308}{100.000}{0.64}{1.36}%
\qsseg{0}{0.000}{85.227}{1.64}{2.36}%
\qsseg{1}{85.577}{100.000}{1.64}{2.36}%
\qsseg{0}{0.000}{79.650}{2.64}{3.36}%
\qsseg{1}{80.000}{98.698}{2.64}{3.36}%
\qsseg{2}{99.048}{100.000}{2.64}{3.36}%
\qsseg{0}{0.000}{79.458}{3.64}{4.36}%
\qsseg{1}{79.808}{94.842}{3.64}{4.36}%
\qsseg{2}{95.192}{100.000}{3.64}{4.36}%
\qsseg{0}{0.000}{72.784}{4.64}{5.36}%
\qsseg{1}{73.134}{100.000}{4.64}{5.36}%
\qsseg{0}{0.000}{70.126}{5.64}{6.36}%
\qsseg{1}{70.476}{78.698}{5.64}{6.36}%
\qsseg{2}{79.048}{82.507}{5.64}{6.36}%
\qsseg{1}{82.857}{86.317}{5.64}{6.36}%
\qsseg{2}{86.667}{89.174}{5.64}{6.36}%
\qsseg{1}{89.524}{92.031}{5.64}{6.36}%
\qsseg{2}{92.381}{93.936}{5.64}{6.36}%
\qsseg{1}{94.286}{95.840}{5.64}{6.36}%
\qsseg{2}{96.190}{96.793}{5.64}{6.36}%
\qsseg{1}{97.143}{97.745}{5.64}{6.36}%
\qsseg{2}{98.095}{98.698}{5.64}{6.36}%
\qsseg{1}{99.048}{100.000}{5.64}{6.36}%
\qsseg{0}{0.000}{69.799}{6.64}{7.36}%
\qsseg{1}{70.149}{100.000}{6.64}{7.36}%
\qsseg{0}{0.000}{66.317}{7.64}{8.36}%
\qsseg{1}{66.667}{93.589}{7.64}{8.36}%
\qsseg{2}{93.939}{100.000}{7.64}{8.36}%
\qsseg{0}{0.000}{63.829}{8.64}{9.36}%
\qsseg{1}{64.179}{100.000}{8.64}{9.36}%
\qsseg{0}{0.000}{62.507}{9.64}{10.36}%
\qsseg{1}{62.857}{89.174}{9.64}{10.36}%
\qsseg{2}{89.524}{100.000}{9.64}{10.36}%
\qsseg{0}{0.000}{60.227}{10.64}{11.36}%
\qsseg{1}{60.577}{81.381}{10.64}{11.36}%
\qsseg{2}{81.731}{98.688}{10.64}{11.36}%
\qsseg{1}{99.038}{100.000}{10.64}{11.36}%
\qsseg{0}{0.000}{57.226}{11.64}{12.36}%
\qsseg{1}{57.576}{81.468}{11.64}{12.36}%
\qsseg{2}{81.818}{93.589}{11.64}{12.36}%
\qsseg{1}{93.939}{100.000}{11.64}{12.36}%
\qsseg{0}{0.000}{55.419}{12.64}{13.36}%
\qsseg{1}{55.769}{100.000}{12.64}{13.36}%
\qsseg{0}{0.000}{54.888}{13.64}{14.36}%
\qsseg{1}{55.238}{89.174}{13.64}{14.36}%
\qsseg{2}{89.524}{94.888}{13.64}{14.36}%
\qsseg{1}{95.238}{100.000}{13.64}{14.36}%
\qsseg{0}{0.000}{54.458}{14.64}{15.36}%
\qsseg{1}{54.808}{84.265}{14.64}{15.36}%
\qsseg{2}{84.615}{96.765}{14.64}{15.36}%
\qsseg{1}{97.115}{100.000}{14.64}{15.36}%
\qsseg{0}{0.000}{49.174}{15.64}{16.36}%
\qsseg{1}{49.524}{90.126}{15.64}{16.36}%
\qsseg{2}{90.476}{95.840}{15.64}{16.36}%
\qsseg{1}{96.190}{97.745}{15.64}{16.36}%
\qsseg{2}{98.095}{98.698}{15.64}{16.36}%
\qsseg{1}{99.048}{100.000}{15.64}{16.36}%
\qsseg{0}{0.000}{45.804}{16.64}{17.36}%
\qsseg{1}{46.154}{80.419}{16.64}{17.36}%
\qsseg{2}{80.769}{90.035}{16.64}{17.36}%
\qsseg{1}{90.385}{93.881}{16.64}{17.36}%
\qsseg{2}{94.231}{96.765}{16.64}{17.36}%
\qsseg{1}{97.115}{97.727}{16.64}{17.36}%
\qsseg{2}{98.077}{98.688}{16.64}{17.36}%
\qsseg{1}{99.038}{100.000}{16.64}{17.36}%
\qsseg{0}{0.000}{43.460}{17.64}{18.36}%
\qsseg{1}{43.810}{77.745}{17.64}{18.36}%
\qsseg{2}{78.095}{100.000}{17.64}{18.36}%
\qsseg{0}{0.000}{43.339}{18.64}{19.36}%
\qsseg{1}{43.689}{59.844}{18.64}{19.36}%
\qsseg{2}{60.194}{75.378}{18.64}{19.36}%
\qsseg{1}{75.728}{90.912}{18.64}{19.36}%
\qsseg{2}{91.262}{100.000}{18.64}{19.36}%
\qsseg{0}{0.000}{40.996}{19.64}{20.36}%
\qsseg{1}{41.346}{68.881}{19.64}{20.36}%
\qsseg{2}{69.231}{90.035}{19.64}{20.36}%
\qsseg{1}{90.385}{100.000}{19.64}{20.36}%
\qsseg{0}{0.000}{39.073}{20.64}{21.36}%
\qsseg{1}{39.423}{76.573}{20.64}{21.36}%
\qsseg{2}{76.923}{86.188}{20.64}{21.36}%
\qsseg{1}{86.538}{90.996}{20.64}{21.36}%
\qsseg{2}{91.346}{94.842}{20.64}{21.36}%
\qsseg{1}{95.192}{97.727}{20.64}{21.36}%
\qsseg{2}{98.077}{100.000}{20.64}{21.36}%
\qsseg{0}{0.000}{36.793}{21.64}{22.36}%
\qsseg{1}{37.143}{68.221}{21.64}{22.36}%
\qsseg{2}{68.571}{80.602}{21.64}{22.36}%
\qsseg{1}{80.952}{91.079}{21.64}{22.36}%
\qsseg{2}{91.429}{93.936}{21.64}{22.36}%
\qsseg{1}{94.286}{95.840}{21.64}{22.36}%
\qsseg{2}{96.190}{97.745}{21.64}{22.36}%
\qsseg{1}{98.095}{98.698}{21.64}{22.36}%
\qsseg{2}{99.048}{100.000}{21.64}{22.36}%
\qsseg{0}{0.000}{30.718}{22.64}{23.36}%
\qsseg{1}{31.068}{48.194}{22.64}{23.36}%
\qsseg{2}{48.544}{63.728}{22.64}{23.36}%
\qsseg{1}{64.078}{77.320}{22.64}{23.36}%
\qsseg{2}{77.670}{87.029}{22.64}{23.36}%
\qsseg{1}{87.379}{94.796}{22.64}{23.36}%
\qsseg{2}{95.146}{100.000}{22.64}{23.36}%
\qsseg{0}{0.000}{30.126}{23.64}{24.36}%
\qsseg{1}{30.476}{39.650}{23.64}{24.36}%
\qsseg{2}{40.000}{49.174}{23.64}{24.36}%
\qsseg{1}{49.524}{57.745}{23.64}{24.36}%
\qsseg{2}{58.095}{62.507}{23.64}{24.36}%
\qsseg{1}{62.857}{66.317}{23.64}{24.36}%
\qsseg{2}{66.667}{69.174}{23.64}{24.36}%
\qsseg{1}{69.524}{72.031}{23.64}{24.36}%
\qsseg{2}{72.381}{74.888}{23.64}{24.36}%
\qsseg{1}{75.238}{77.745}{23.64}{24.36}%
\qsseg{2}{78.095}{80.602}{23.64}{24.36}%
\qsseg{1}{80.952}{82.507}{23.64}{24.36}%
\qsseg{2}{82.857}{84.412}{23.64}{24.36}%
\qsseg{1}{84.762}{86.317}{23.64}{24.36}%
\qsseg{2}{86.667}{87.269}{23.64}{24.36}%
\qsseg{1}{87.619}{88.221}{23.64}{24.36}%
\qsseg{2}{88.571}{89.174}{23.64}{24.36}%
\qsseg{1}{89.524}{90.126}{23.64}{24.36}%
\qsseg{2}{90.476}{91.079}{23.64}{24.36}%
\qsseg{1}{91.429}{92.031}{23.64}{24.36}%
\qsseg{2}{92.381}{92.983}{23.64}{24.36}%
\qsseg{1}{93.333}{93.936}{23.64}{24.36}%
\qsseg{2}{94.286}{94.888}{23.64}{24.36}%
\qsseg{1}{95.238}{95.840}{23.64}{24.36}%
\qsseg{2}{96.190}{96.793}{23.64}{24.36}%
\qsseg{1}{97.143}{97.745}{23.64}{24.36}%
\qsseg{2}{98.095}{98.698}{23.64}{24.36}%
\qsseg{1}{99.048}{100.000}{23.64}{24.36}%
\qsseg{0}{0.000}{29.953}{24.64}{25.36}%
\qsseg{1}{30.303}{55.711}{24.64}{25.36}%
\qsseg{2}{56.061}{76.923}{24.64}{25.36}%
\qsseg{1}{77.273}{82.983}{24.64}{25.36}%
\qsseg{2}{83.333}{89.044}{24.64}{25.36}%
\qsseg{1}{89.394}{93.589}{24.64}{25.36}%
\qsseg{2}{93.939}{95.105}{24.64}{25.36}%
\qsseg{1}{95.455}{96.620}{24.64}{25.36}%
\qsseg{2}{96.970}{98.135}{24.64}{25.36}%
\qsseg{1}{98.485}{100.000}{24.64}{25.36}%
\qsseg{0}{0.000}{25.612}{25.64}{26.36}%
\qsseg{1}{25.962}{40.035}{25.64}{26.36}%
\qsseg{2}{40.385}{50.612}{25.64}{26.36}%
\qsseg{1}{50.962}{57.342}{25.64}{26.36}%
\qsseg{2}{57.692}{62.150}{25.64}{26.36}%
\qsseg{1}{62.500}{66.958}{25.64}{26.36}%
\qsseg{2}{67.308}{71.765}{25.64}{26.36}%
\qsseg{1}{72.115}{76.573}{25.64}{26.36}%
\qsseg{2}{76.923}{81.381}{25.64}{26.36}%
\qsseg{1}{81.731}{85.227}{25.64}{26.36}%
\qsseg{2}{85.577}{89.073}{25.64}{26.36}%
\qsseg{1}{89.423}{92.919}{25.64}{26.36}%
\qsseg{2}{93.269}{94.842}{25.64}{26.36}%
\qsseg{1}{95.192}{96.765}{25.64}{26.36}%
\qsseg{2}{97.115}{98.688}{25.64}{26.36}%
\qsseg{1}{99.038}{100.000}{25.64}{26.36}%
\qsseg{3}{0.000}{96.793}{28.24}{28.96}%
\qsseg{4}{97.143}{100.000}{28.24}{28.96}%
\qsseg{3}{0.000}{94.888}{29.24}{29.96}%
\qsseg{4}{95.238}{96.793}{29.24}{29.96}%
\qsseg{5}{97.143}{98.698}{29.24}{29.96}%
\qsseg{4}{99.048}{100.000}{29.24}{29.96}%
\qsseg{3}{0.000}{93.881}{30.24}{30.96}%
\qsseg{4}{94.231}{100.000}{30.24}{30.96}%
\qsseg{3}{0.000}{91.958}{31.24}{31.96}%
\qsseg{4}{92.308}{95.804}{31.24}{31.96}%
\qsseg{5}{96.154}{97.727}{31.24}{31.96}%
\qsseg{4}{98.077}{100.000}{31.24}{31.96}%
\qsseg{3}{0.000}{84.412}{32.24}{32.96}%
\qsseg{4}{84.762}{100.000}{32.24}{32.96}%
\qsseg{3}{0.000}{73.688}{33.24}{33.96}%
\qsseg{4}{74.038}{100.000}{33.24}{33.96}%
\qsseg{3}{0.000}{71.765}{34.24}{34.96}%
\qsseg{4}{72.115}{100.000}{34.24}{34.96}%
\qsseg{3}{0.000}{59.650}{35.24}{35.96}%
\qsseg{4}{60.000}{82.150}{35.24}{35.96}%
\qsseg{5}{82.500}{100.000}{35.24}{35.96}%
\qsseg{3}{0.000}{46.027}{36.24}{36.96}%
\qsseg{4}{46.377}{88.056}{36.24}{36.96}%
\qsseg{5}{88.406}{100.000}{36.24}{36.96}%
\qsseg{3}{0.000}{41.958}{37.24}{37.96}%
\qsseg{4}{42.308}{77.535}{37.24}{37.96}%
\qsseg{5}{77.885}{100.000}{37.24}{37.96}%
\qsseg{3}{0.000}{30.126}{38.24}{38.96}%
\qsseg{4}{30.476}{55.840}{38.24}{38.96}%
\qsseg{5}{56.190}{72.983}{38.24}{38.96}%
\qsseg{4}{73.333}{83.460}{38.24}{38.96}%
\qsseg{5}{83.810}{92.983}{38.24}{38.96}%
\qsseg{4}{93.333}{100.000}{38.24}{38.96}%
\qsseg{6}{0.000}{90.996}{40.84}{41.56}%
\qsseg{7}{91.346}{98.688}{40.84}{41.56}%
\qsseg{8}{99.038}{100.000}{40.84}{41.56}%
\qsseg{6}{0.000}{67.269}{41.84}{42.56}%
\qsseg{7}{67.619}{98.698}{41.84}{42.56}%
\qsseg{8}{99.048}{100.000}{41.84}{42.56}%
