# Supplementary material for: Off the Driven Path: Transferable Road Understanding in Driving VLAs
Source: arXiv:2611.33878 source file (2026-11-25)
Supplement: Supplementary file 3 [file meta.tex]

\scaset{boston}{n}{95}%
\scaset{boston}{km}{33.333}%
\scaset{boston-k1}{mean}{1.0}%
\scaset{boston-k2}{mean}{1.6}%
\scaset{boston-k4}{mean}{2.2}%
\scaset{boston-all}{mean}{2.9}%
\scaset{pittsburgh}{n}{118}%
\scaset{pittsburgh}{km}{50.000}%
\scaset{pittsburgh-k1}{mean}{1.0}%
\scaset{pittsburgh-k2}{mean}{1.7}%
\scaset{pittsburgh-k4}{mean}{2.5}%
\scaset{pittsburgh-all}{mean}{3.6}%
\scaset{lasvegas}{n}{116}%
\scaset{lasvegas}{km}{16.667}%
\scaset{lasvegas-k1}{mean}{1.0}%
\scaset{lasvegas-k2}{mean}{1.8}%
\scaset{lasvegas-k4}{mean}{3.1}%
\scaset{lasvegas-all}{mean}{16.5}%
\scaset{singapore}{n}{86}%
\scaset{singapore}{km}{50.000}%
\scaset{singapore-k1}{mean}{1.0}%
\scaset{singapore-k2}{mean}{1.6}%
\scaset{singapore-k4}{mean}{2.3}%
\scaset{singapore-all}{mean}{2.7}%
